# Supplementary material for: GameAnything: From Any Inspirations to Playable Game Worlds
Source: arXiv:2611.29238 source file (2026-11-22)
Supplement: Supplementary file 1 [file ablation_refinement.tex]

% Numbers from data/experiment_tracker/ablation/analysis/ablation_results.md (Exp 1, 2026-11-20). Hand-written.
\begin{tabular}{@{}lccc cc c cc c@{}}
\toprule
 & & & & \multicolumn{3}{c}{\textbf{Claude Sonnet 5.5}} & \multicolumn{3}{c}{\textbf{DeepSeek V4.1 Flash}} \\
\cmidrule(lr){5-7}\cmidrule(lr){8-10}
\textbf{Setting} & \textbf{Min.} & \textbf{Critic} & \textbf{Memory} & \textbf{Overall} & $\Delta$ [95\% CI] & \textbf{\$} & \textbf{Overall} & $\Delta$ [95\% CI] & \textbf{\$} \\
\midrule
R0 (native) & -- & -- & -- & 65.0 & -- & -- & 59.0 & -- & -- \\
Extra budget only & 60 & \tabno & \tabno & 65.3 & +0.3 [$-$1.9, +2.6] & 0.49 & 59.0 & +0.0 [$-$3.3, +3.2] & 0.14 \\
Critic, no memory & 60 & \tabyes & \tabno & 65.7 & +0.7 [$-$3.6, +4.8] & 1.16 & 57.1 & $-$1.9 [$-$5.8, +1.7] & 0.40 \\
Critic + memory & 60 & \tabyes & \tabyes & 65.1 & +0.1 [$-$3.2, +3.5] & 1.20 & 55.7 & $-$3.3 [$-$8.8, +1.4] & 0.52 \\
R1 of Table~\ref{tab:refinement_results}$^{\dagger}$ & 40 & \tabyes & \tabno & 65.8 & +0.8 [$-$2.4, +3.9] & 0.94 & 57.5 & $-$1.5 [$-$4.3, +1.5] & 0.36 \\
\midrule
\multicolumn{4}{@{}l}{Memory effect (critic + memory $-$ critic, no memory)} & & $-$0.6 [$-$4.1, +2.9] & & & $-$1.4 [$-$7.7, +4.2] & \\
\multicolumn{4}{@{}l}{Critic + memory $-$ extra budget only} & & $-$0.2 [$-$3.4, +3.0] & & & $-$3.3 [$-$8.4, +0.8] & \\
\bottomrule
\end{tabular}
